# Supplementary material for: Magnetism in Two-Dimensional Ilmenenes: Intrinsic Order and Strong Anisotropy
Source: arXiv:2211.01732 source file (2022-11-03)
Supplement: Supplementary file 1 [file Supplementary_Information.pdf]

# Supplementary Information: Magnetism in Two-Dimensional Ilmenenes: Intrinsic Order and Strong Anisotropy

R.H Aguilera-del-Toro[1−2], M. Arruabarrena[2], A. Leonardo[1−3], and A. Ayuela[1−2]

[1]*Donostia International Physics Center (DIPC),*

*20018 Donostia, Spain*

[2]*Centro de Física de Materiales - Materials Physics Center (CFM-MPC),*

*20018 Donostia, Spain*

*and*

[3]*EHU Quantum Center,*

*Universidad del País Vasco/Euskal Herriko Unibertsitatea UPV/EHU, Leioa, Spain*

## I. COULOUMB INTERACTION IN OXIDES: DFT+U METHOD

A careful consideration of Coulomb interactions is important for calculations of oxides involving 3d transition metals. DFT calculations using standard generalized gradient approximations are known to localize the 3d electrons of the transition metals in oxides less than expected, and to properly describe their electronic and magnetic properties, corrections such as the DFT+U method are needed. In this work, we use the Dudarev formulation for GGA+U, in which a single effective correction term $U_{eff}$ =U-J is applied to the 3d orbitals of the transition metals, which includes the coulomb and exchange interactions. The $U_{eff}$ parameters are collected in table I for some transition metals and brass metals that are in the third row of the periodic table . These values have been taken from other works[1–4] in which good results were reported for molecules and bulk systems. In several works, the use of U parameters is applied not only to transition metal atoms, but also to oxygen electrons[5–8]. To check the validity of our DFT+U results, we calculate the density of states with and without applying the correction parameter on oxygen, and use a hybrid calculation as benchmark. In Figure S1 we show the density of states for the three following cases: (a) without adding U parameter in oxygen, (c) including the U parameter in oxygen, and (b) an hybrid-HSE06 calculation. We first note that the HOMO-LUMO gap is more similar to the hybrid calculation when the term U for oxygen is included. Furthermore, the density of states for these last two cases are in better agreement, and show a larger localization of the cobalt and oxygen electrons near the Fermi level, a trend that is not observed for the calculation in which the U parameter was not included in the oxygen atoms.

Table S I. Valence electron states, and U parameters employed on each element of the TM titanates.

| Element | Valence states | U |
|---|---|---|
| O | 2s, 2p | 6.6 |
| Ti | 3p, 3d, 4s | 3.9 |
| V | 3p, 3d, 4s | 3.5 |
| Cr | 3p, 3d, 4s | 3.5 |
| Mn | 3p, 3d, 4s | 4.0 |
| Fe | 3d, 4s | 4.0 |
| Co | 3d, 4s | 4.5 |
| Ni | 3d, 4s | 4.5 |
| Cu | 3d, 4s | 5.0 |
| Zn | 3d, 4s | 5.0 |

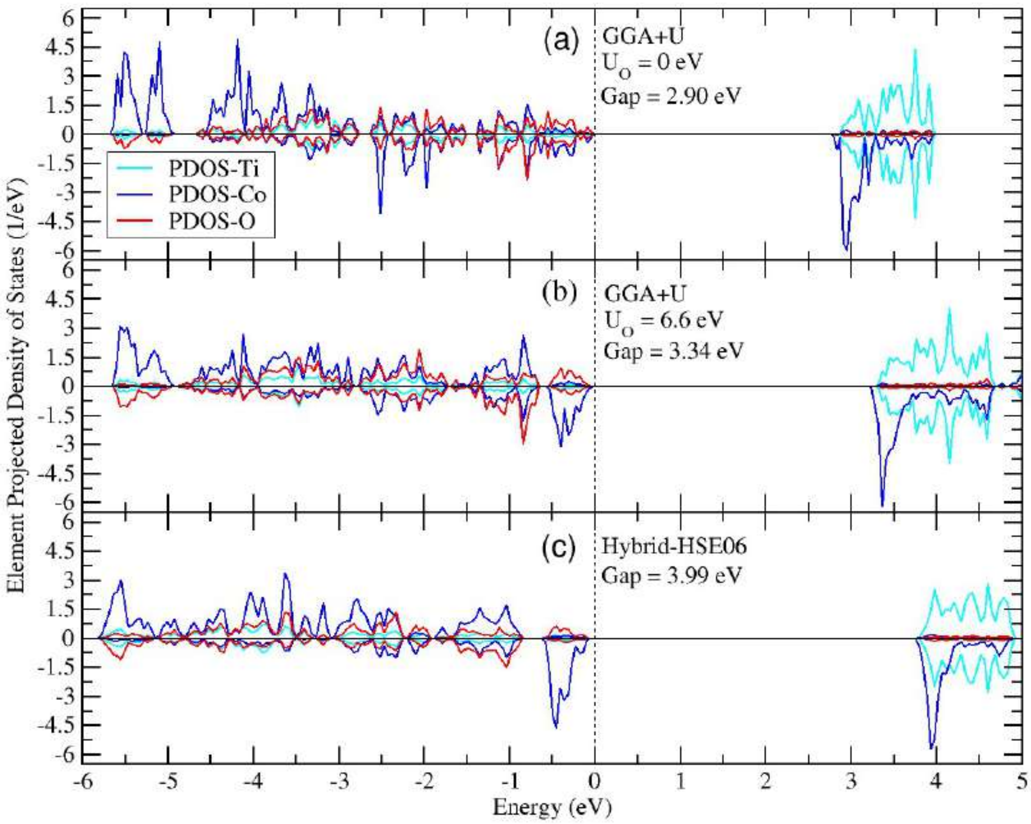


Fig. S 1. Projected density of states of cobalt titanate (a) without using a U parameter in oxygen, (c) adding U=6.6 eV in oxygen, and (b) in the hybrid HSE06 approach.

## II. RELAXED STRUCTURES

In this work, two families of different titanate layers were tested: those terminated in transition metals and those terminated in titanium (see Fig. S2). For all the compounds under analysis, the transition metal-terminated layers are found to be more stable, with energy differences between 1.0 and 4.0 eV with respect to their Ti-ended counterparts. The structures for the Cr and Cu ilmenenes are shown in Fig. S3. As mentioned in the main text, these two compounds differ significantly from the rest of the titanates because they present notable structural deformations. This deformation is more evident in the chromium ilmenene, where the sub-lattice formed by the titanium atoms presents a certain roughness, while in the rest of the layers a fully flat graphene-like hexagonal sublattice of Ti ions is observed. We advance that these deformations have a Jahn-Teller type origin, to be discussed below.

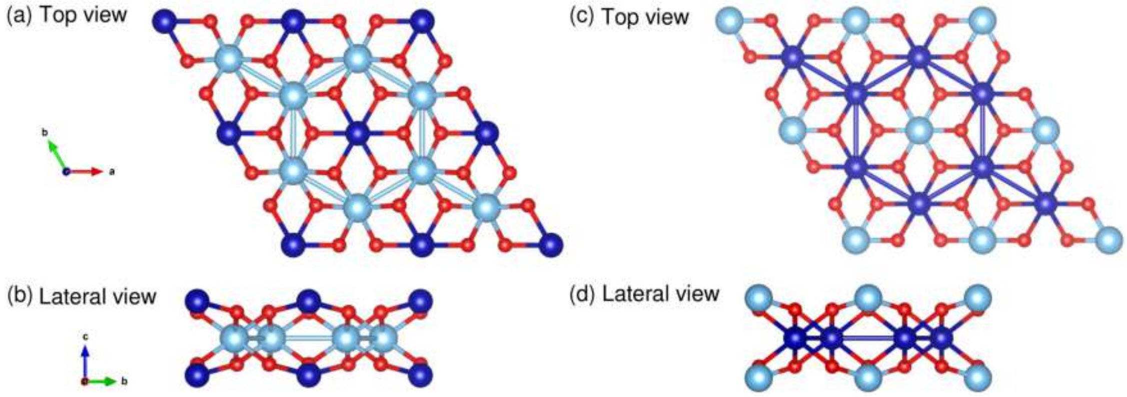


Fig. S 2. Distorted ilmenene structures of (a,b) transition metal terminated layer and (c,d) titanium terminated sheet. For all the analyzed compounds, the transition metal termination was found to be more stable.

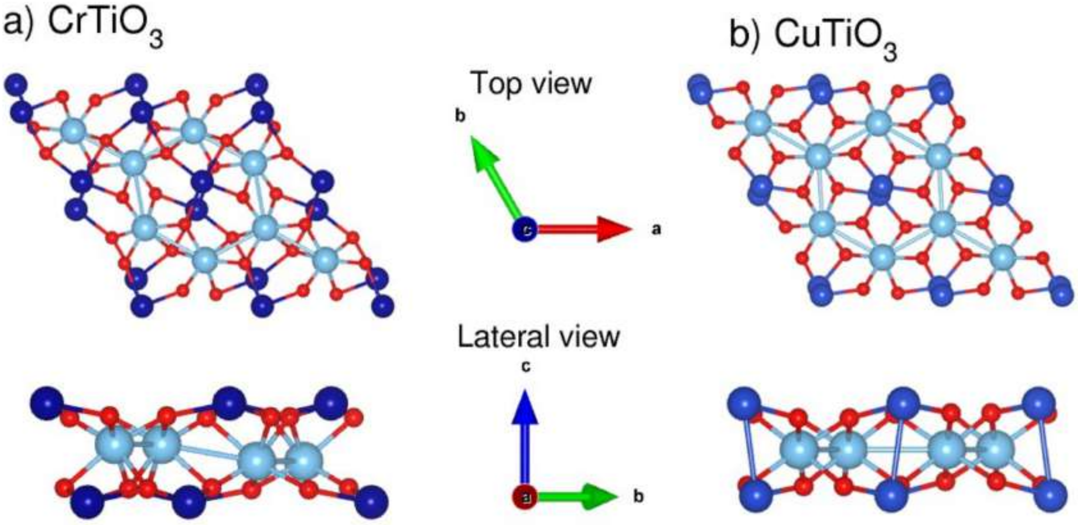


Fig. S 3. Ilemene structures for (a) chromium and (b) copper titanates.

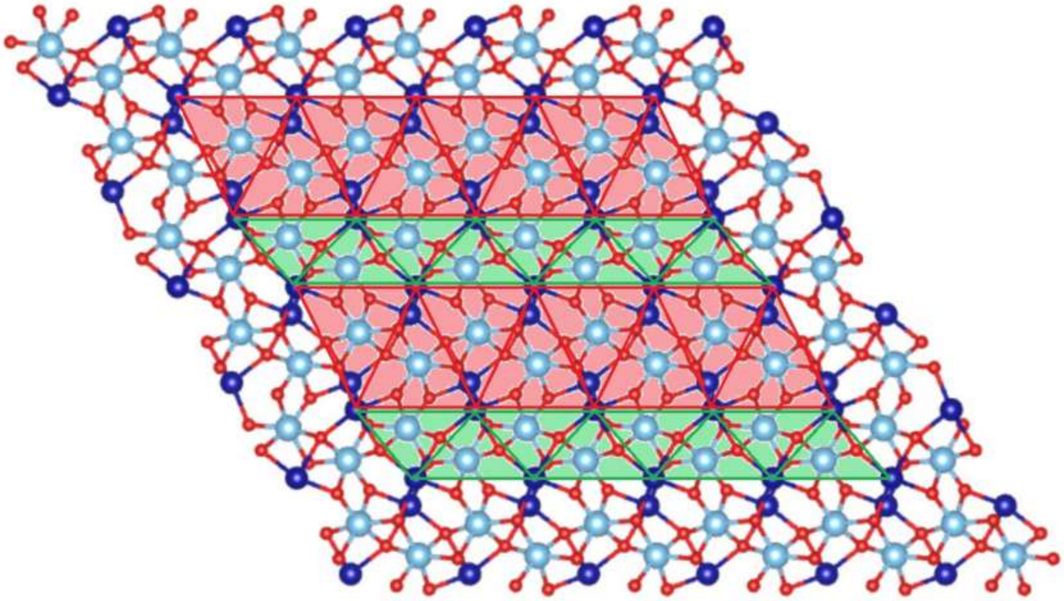

Fig. S 4. Structure of the chromium ilmenene. In red and green, the two different triangle ribbons are depicted. The structural deformation is most notable in this compound, that shows one dimensional anisotropy as in other interesting 2D materials like phosphorene.

## III. ELECTRONIC STRUCTURE: BANDS AND LEVEL SCHEMES

We collect the projected densities of states on an atom of each chemical species in Figures S5-S7. More interestingly, Figures S8-S10 show the band structures projected on the electronic orbitals with the transition metal atom ranging from V to Zn. We divide the analysis of ilmenes into three categories: below half filling (V, Cr and Mn), above half filing (Fe, Co and Ni), and just below full filling (brass metals, Zu and Zn).

(i) In the case of the below half filling ilmenenes (Fig. S8), the $d_{xz}$, $d_{yz}$ and $d_{z^2}$ orbitals with an out-of-plane component are the first to be occupied, while the in-plane ones are the least stable. For the chromium ilmenene, the $d_{xz}$ and $d_{yz}$ orbitals are splitted: the $d_{xy}$ and $d_{x^2-y^2}$ orbitals are highly splitted, with the $d_{x^2-y^2}$ orbital being occupied, and the dxy orbital unoccupied. This splitting is the source of Jahn-Teller like distortions for Cr ilmenenes.

(ii) Ilemenenes above half filling (Fig. S9) have the down-spin part of the orbitals coming into play. For iron ilmenene, the first orbital to fill is $d_{z^2}$, while in the case of cobalt, due to degenerate orbitals, the system prefers to fill the $d_{xz}$ and $d_{yz}$ orbitals first. For nickel titanate, the $d_{z^2}$ orbital is again filled first, while the others are partially filled. This kind of alternance gives rise to odd-even trends when the levels are being occupied in going from Fe to Ni oxide ilmenenes.

(iii) Finally, in Fig. S10, copper ilmenene shows a similar behavior to the chromium ilmenene: the $d_{xz}$ and $d_{yz}$ orbitals split, as do the $d_{xy}$ and $d_{x^2-y^2}$ orbitals, with the $d_{xy}$ orbital being the unoccupied one. The zinc titanate ilmenene with a $d^{10}$ electronic configuration has all orbitals occupied, and is spin compensated.

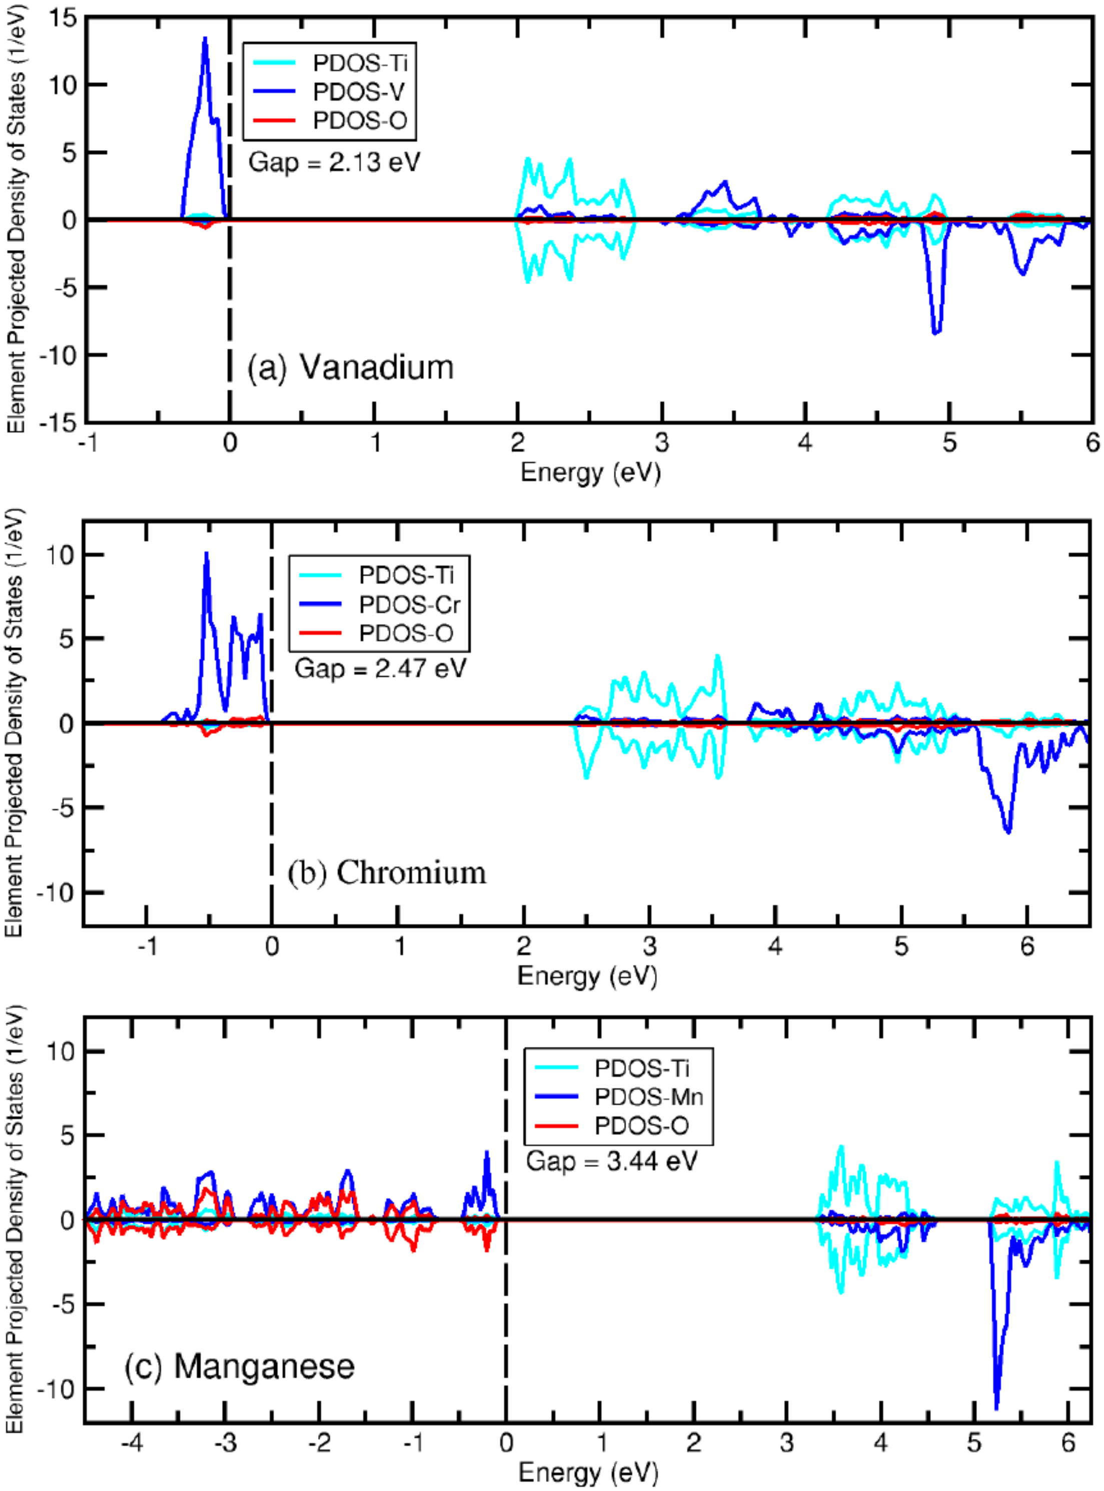


Fig. S 5. Element-projected density of states (DOS) on a atom of each atomic species. Transition metal is denoted in blue, titanium in cyan, and oxygen in red.

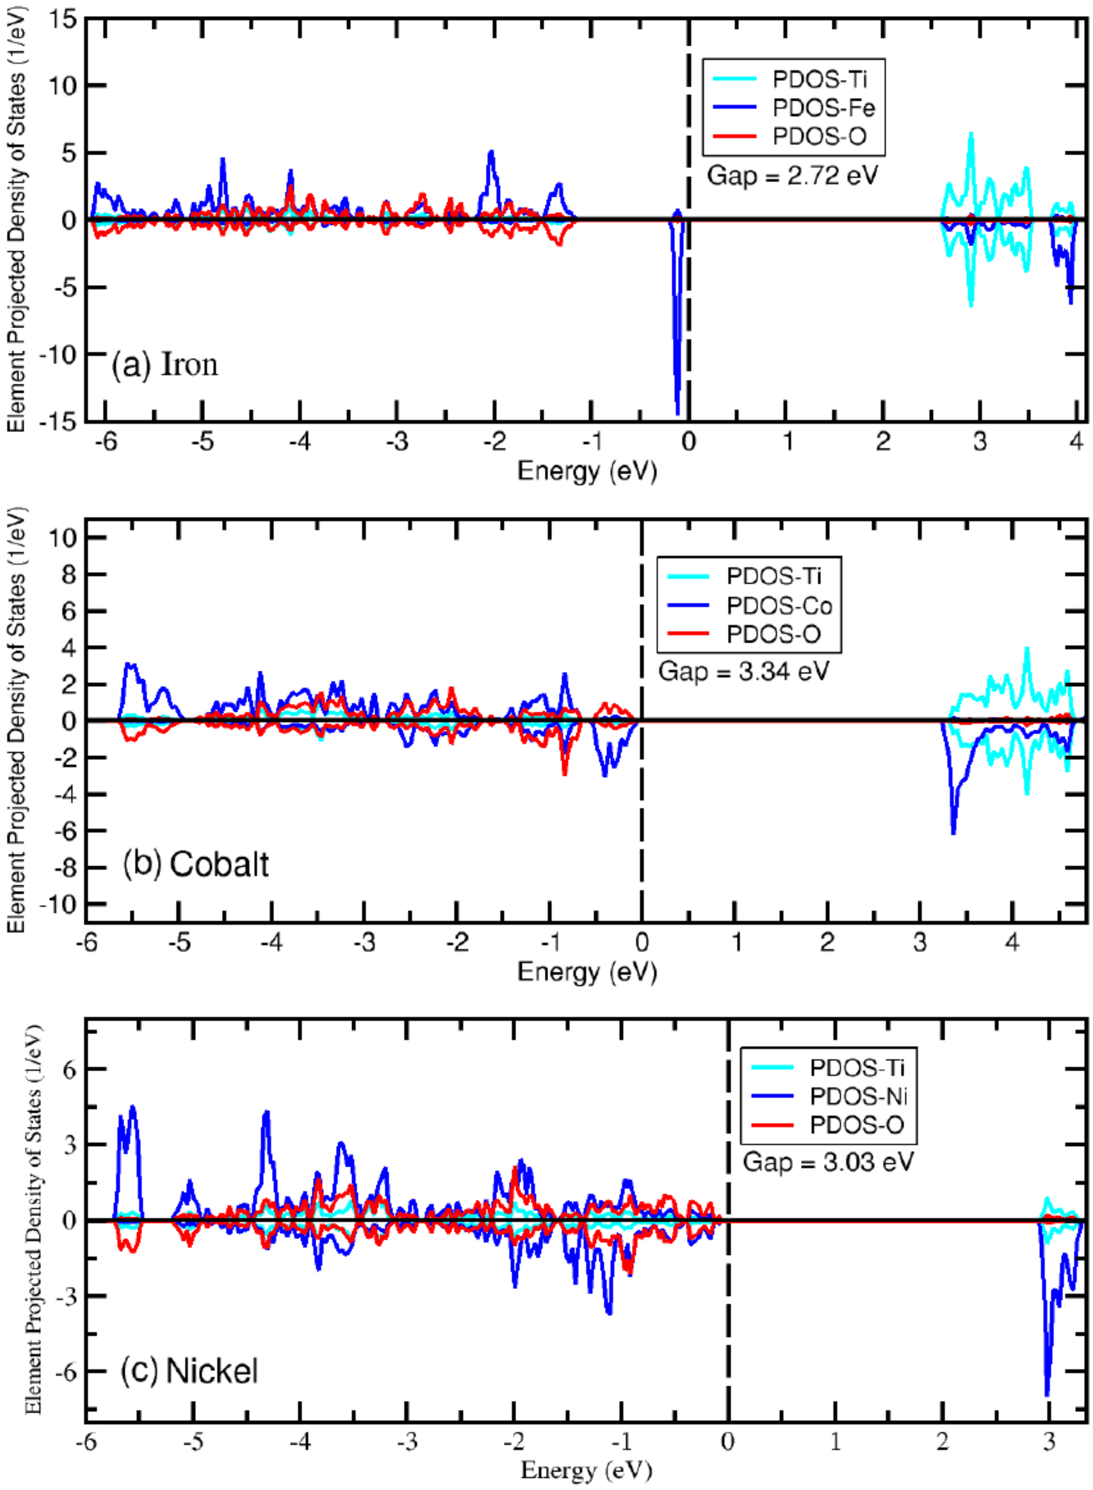


Fig. S 6. Element-projected density of states (DOS) on a atom of each atomic species. Colors follow the caption of previous figure.

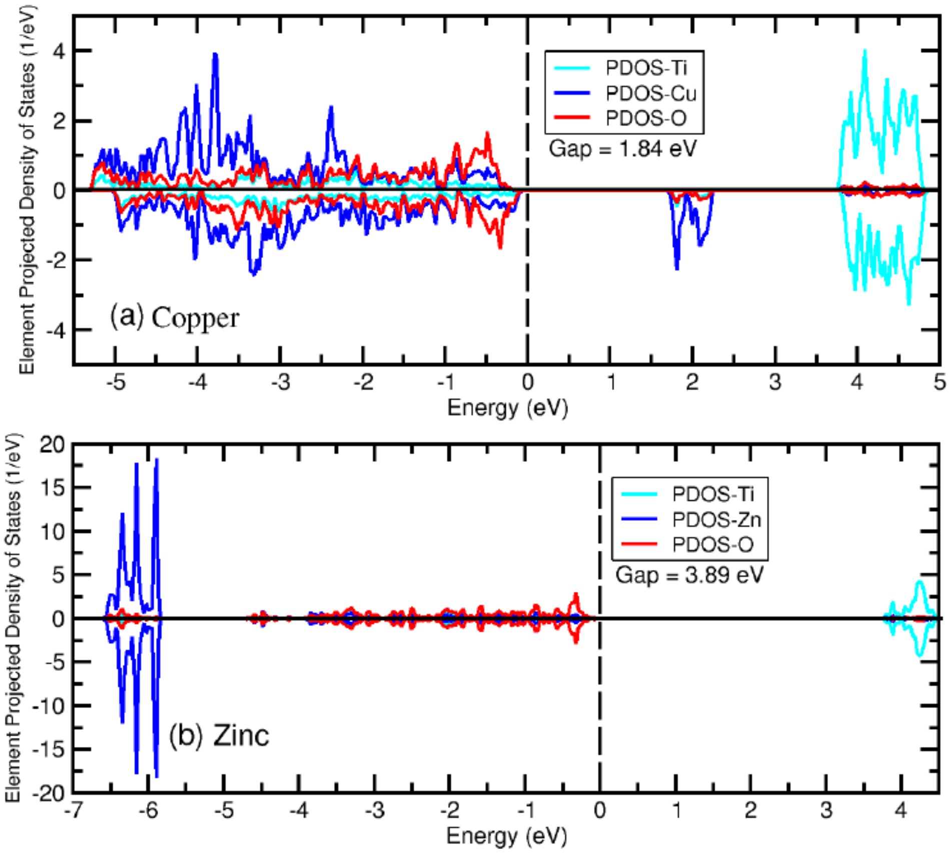


Fig. S 7. Element-projected density of states (DOS) on a atom of each atomic species. Colors follow the caption of figures above.

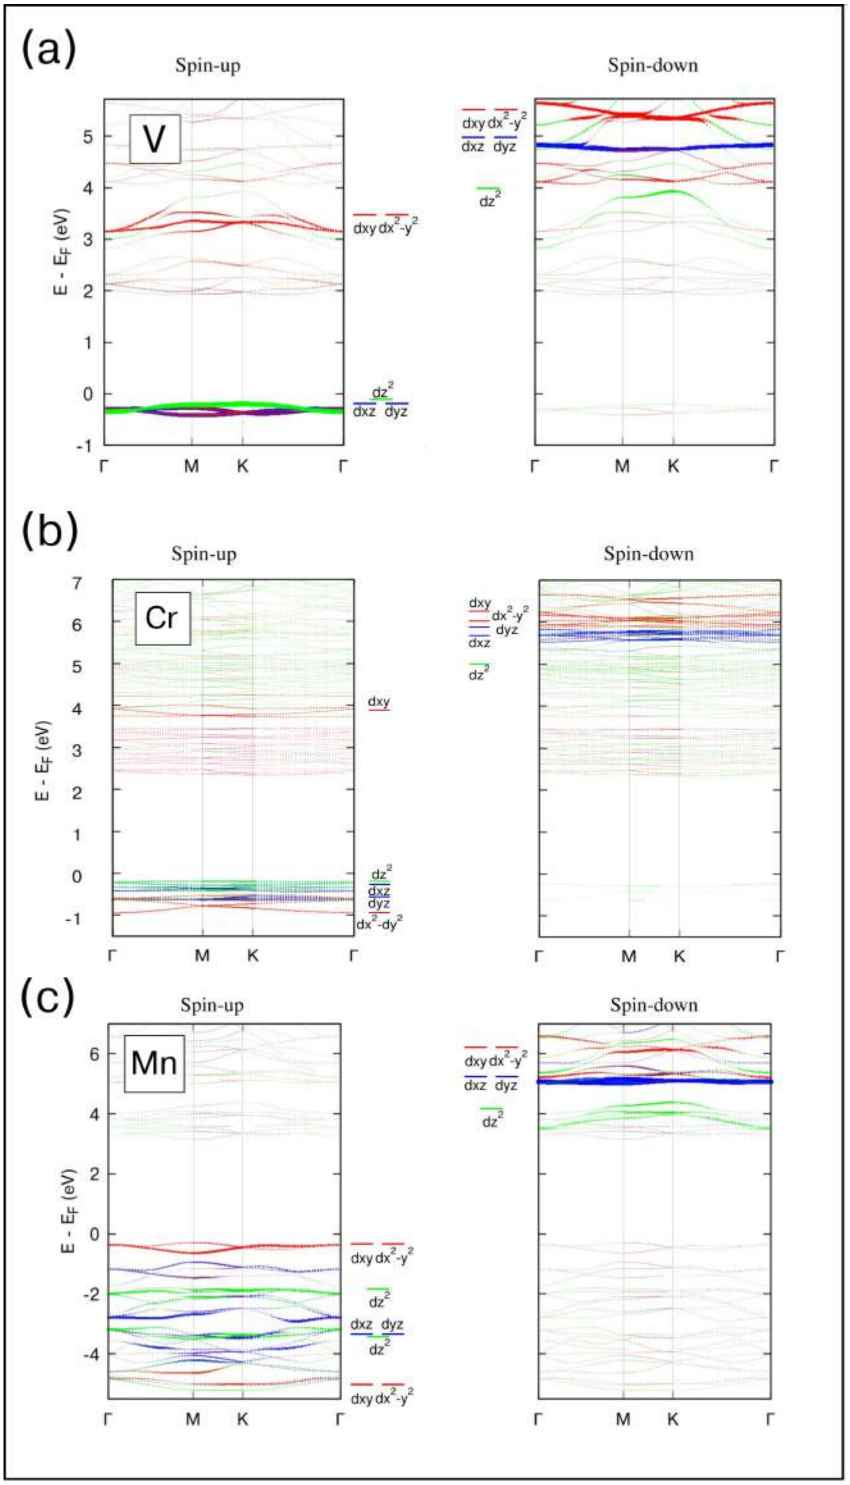


Fig. S 8. Electronic band structure and PDOS for the ilmenenes below half-filling. Vanadium titanate, chromium titanate and manganese titanate are displayed in panels (a), (b) and (c), respectively.

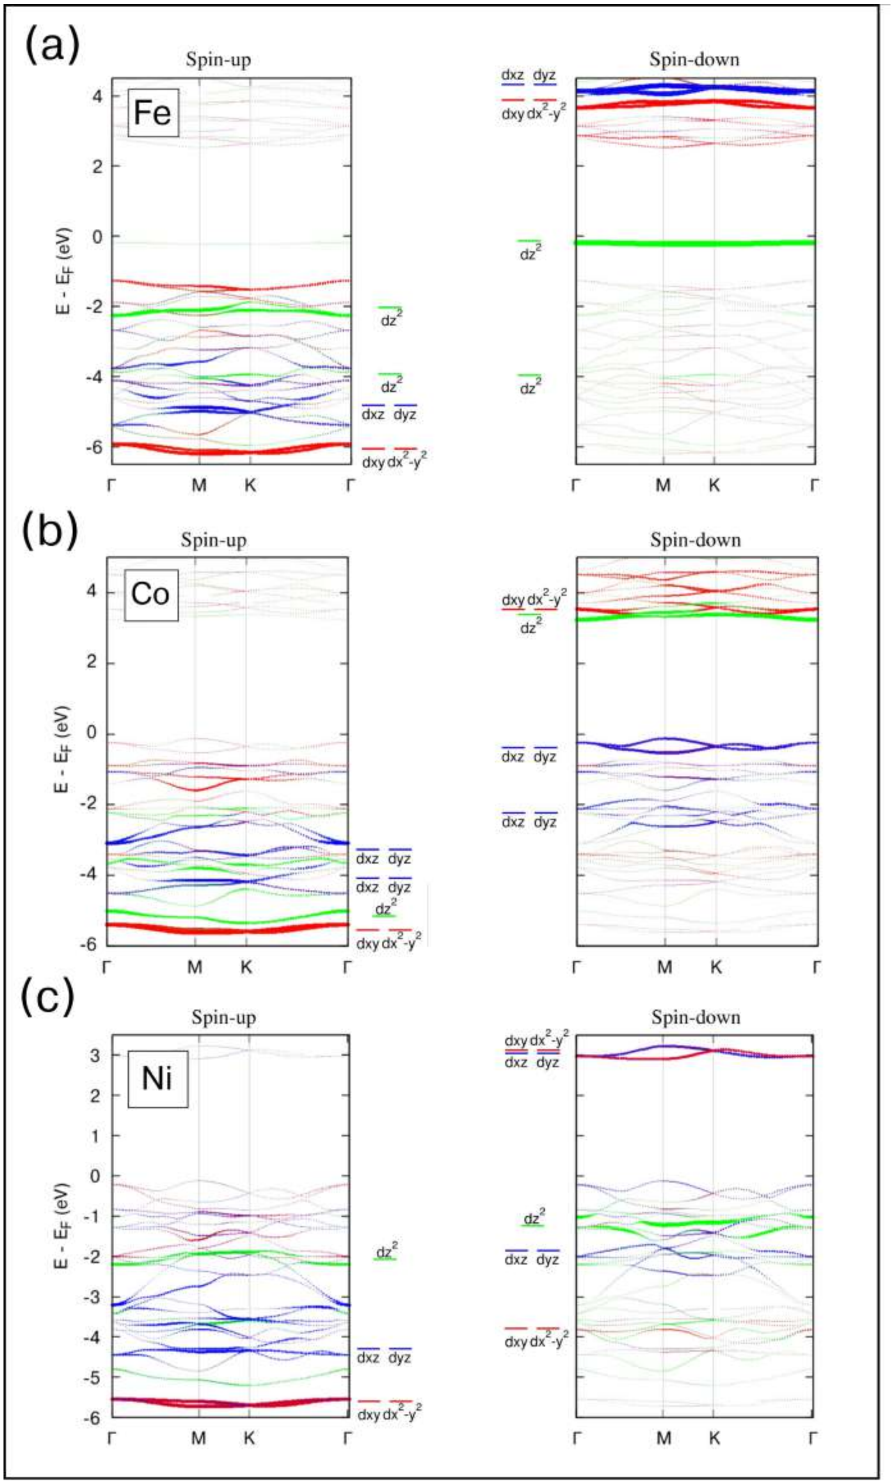


Fig. S 9. Electronic band structure and PDOS for the ilmenenes above half-filling. Iron titanate, cobalt titanate and nickel titanate are displayed in panels (a), (b) and (c), respectively.

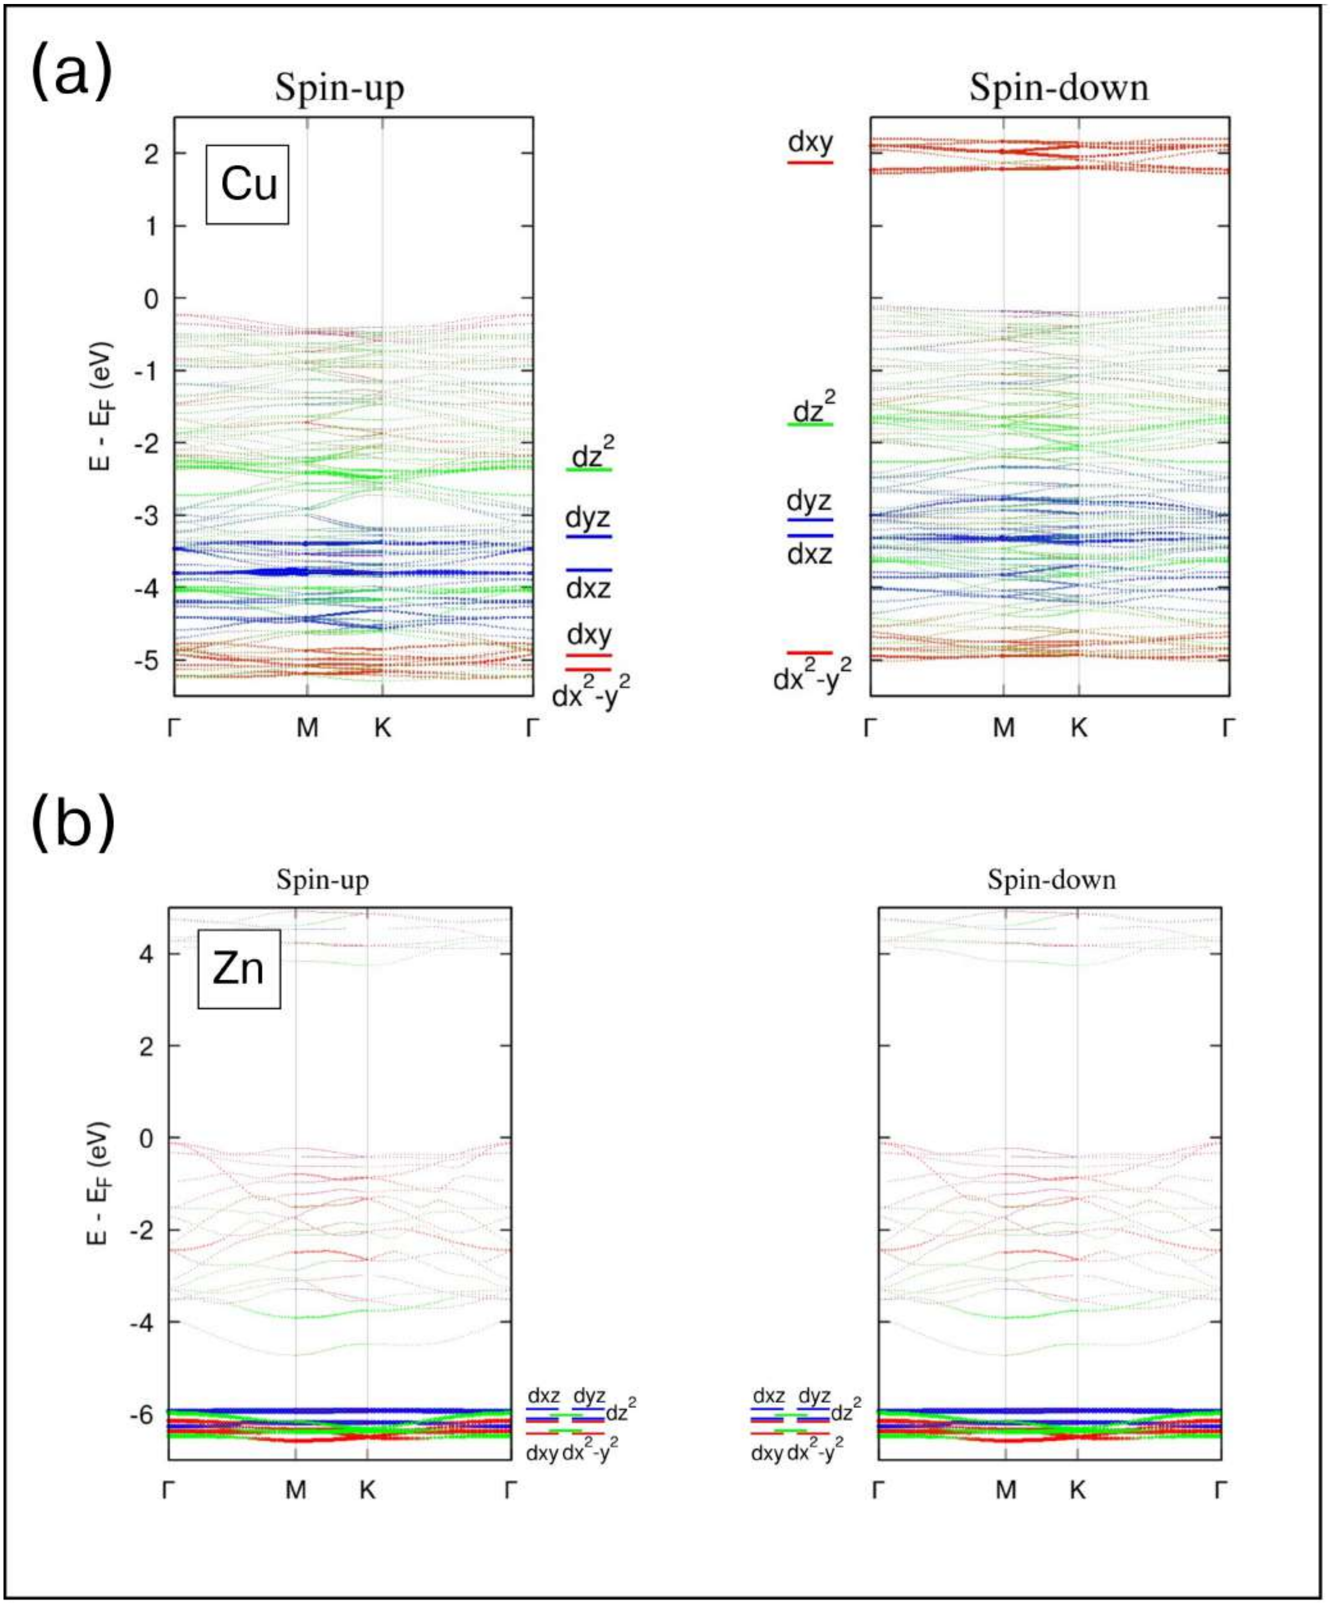


Fig. S 10. Electronic band structure and PDOS of the brass metal ilmenenes copper titanate (panel (a)) and zinc titanate (panel (b)).

## IV. CALCULATION OF THE MAGNETIC COUPLING CONSTANTS

To compute the magnetic coupling between the transition metal atoms in the ilmenene layers, we consider the Heisenberg Hamiltonian

$$H = -\sum_{ij} J_{ij} \tilde{\mathbf{S}}_{\mathbf{i}} \cdot \tilde{\mathbf{S}}_{\mathbf{j}}. \tag{1}$$

Solving for the four main magnetic configurations in Fig. 4 of the main text yields the following energies

$$E_{FM} = -(+J_1 + 6J_2) \cdot \tilde{S}^2 \tag{2}$$

$$E_{AFM-1} = -(-J_1 + 6J_2) \cdot \tilde{S}^2 \tag{3}$$

$$E_{AFM-2} = -(-J_1 - 6J_2) \cdot \tilde{S}^2, \tag{4}$$

where the $\tilde{S}$ is the pseudospin of each isolated atomic species (e.g: $\tilde{S} = 3/2$ for Co), and the $J_i$ (with $i = 1$ and 2) are the inter-layer ($i = 1$) and intra-layer ($i = 2$) magnetic couplings schematically depicted in Fig. 5 of the main text. The magnetic couplings can then be computed from the energy differences $\Delta E_1 = E_{FM} - E_{AFM_1}$ and $\Delta E_2 = E_{AFM_2} - E_{AFM_1}$:

$$J_1 = \frac{\Delta E_1}{2\tilde{S}^2} \tag{5}$$

$$J_2 = \frac{-\Delta E_2}{12\tilde{S}^2}. \tag{6}$$

## V. MAGNETIC CONFIGURATIONS AND EXCITATIONS

In the main text we have discussed three different magnetic configurations. We found that, except for copper and zinc ilmenenes, in which the ground states are respectively ferromagnetic and spin compensated, the ilmenenes present an antiferromagnetic coupling (AFM-1) between transition metal atoms on both layer sides. Nevertheless, due to the large size of our magnetic cell, it is possible to access other types of magnetic configurations. In panels (a) to (h) of Fig. S11, we show other eight possible ways in which the local magnetic moments can be coupled. Their energy differences with respect to the ground state are displayed in Fig. S11(i). The figure collects the map of the excitation energies for other magnetic couplings. As we already discussed in the electronic properties, we find that there are three regions: (i) TM below half-filled, (ii) TM above half-filled and (iii) brass-metals. Overall, the energy differences decrease with the atomic number, with the exception of cobalt ilmenene, that presents a considerable increase for most of the magnetic configurations. Copper ilmenene, as discussed throughout the main text, presents a ferromagnetic ground state.

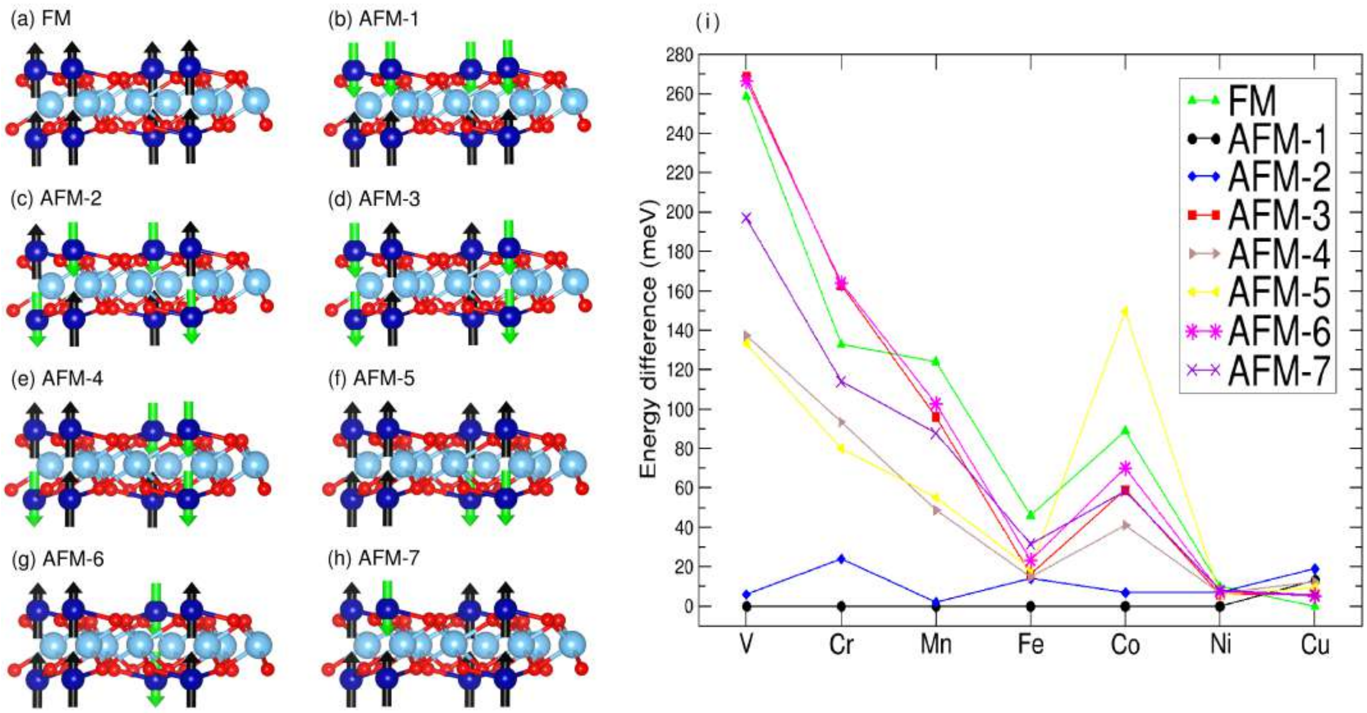


Fig. S 11. (a-h) Magnetic isomers of the TM ilmenenes. (i) Energy differences between each magnetic configuration and the AFM-1 ground state. In the case of the copper ilmenene, this difference is computed with respect to the ferromagnetic ground state.

---


[1] F. Aguilera-Granja and A. Ayuela, Magnetism and distortions in two-dimensional transition-metal dioxides: On the quest for intrinsic magnetic semiconductor layers, The Journal of Physical Chemistry C **124**, 2634 (2020).

[2] E. B. Linscott, D. J. Cole, M. C. Payne, and D. D. O'Regan, Role of spin in the calculation of Hubbard $U$ and Hund's $J$ parameters from first principles, Phys. Rev. B **98**, 235157 (2018).

[3] H. J. Kulik and N. Marzari, Transition-metal dioxides: A case for the intersite term in hubbard-model functionals, The Journal of Chemical Physics **134**, 094103 (2011).

[4] M. Cococcioni and S. de Gironcoli, Linear response approach to the calculation of the effective interaction parameters in the LDA + U method, Phys. Rev. B **71**, 035105 (2005).

[5] B. J. Morgan and G. W. Watson, Polaronic trapping of electrons and holes by native defects in anatase $TiO_2$, Phys. Rev. B **80**, 233102 (2009).

[6] X. Huang, S. K. Ramadugu, and S. E. Mason, Surface-Specific DFT + U Approach Applied to $\alpha$-$Fe_2O_3$(0001), The Journal of Physical Chemistry C **120**, 4919 (2016).

[7] L. Jiang, S. V. Levchenko, and A. M. Rappe, Rigorous definition of oxidation states of ions in solids, Phys. Rev. Lett. **108**, 166403 (2012).

[8] G. Y. Gou, J. W. Bennett, H. Takenaka, and A. M. Rappe, Post density functional theoretical studies of highly polar semiconductive $Pb(Ti_{1-x}Ni_x)O_{3-x}$ solid solutions: Effects of cation arrangement on band gap, Phys. Rev. B **83**, 205115 (2011).
